# Supplementary material for: MedSTP: Preserving Subspace and Transition Evidence for Medical VQA Token Pruning
Source: arXiv:2610.22751 source file (2026-10-15)
Supplement: Supplementary file 1 [file metric.tex]

\section{Metrics and Reporting Protocol}
\label{sec:supp-metric}

All pruning methods are evaluated with frozen backbones and identical prompts, insertion points, and retained-token budgets. A keep ratio of 10\% retains one tenth of the visual tokens and is used for the main tables. A keep ratio of 5\% is the more aggressive setting reported here, corresponding to 95\% visual-token pruning.

\paragraph{Accuracy.}
Accuracy is reported as the percentage of evaluated VQA instances answered correctly. The Avg. column is the overall accuracy across all evaluated instances in a dataset. Group columns report the same correctness metric restricted to one group in Table~\ref{tab:supp-dataset-groups}.

\paragraph{KL divergence.}
KL measures how far the answer distribution under pruning moves from the corresponding full-token answer distribution. Lower KL indicates that the compact visual-token subset better preserves the full-token model behavior, even when the final top answer is unchanged.

\paragraph{Uncertainty.}
Each table entry is reported with a bootstrap standard error when available. Small groups such as SLAKE-PO and OmniMedVQA-ES should be read with this uncertainty in mind, while the Avg. and KL columns provide more stable aggregate views.
