# Supplementary material for: MedSTP: Preserving Subspace and Transition Evidence for Medical VQA Token Pruning
Source: arXiv:2610.22751 source file (2026-10-15)
Supplement: Supplementary file 2 [file 7_appendix.tex]

\section{Additional 5\% Keep Ratio Results}
\label{sec:appendix-five-percent}

Tables~\ref{tab:slake-appendix-five} and~\ref{tab:omnimed-appendix-five} report the 5\% keep ratio results corresponding to the main result tables. The column order matches the main text: group accuracies first, followed by the overall average accuracy and KL divergence from the full token answer distribution. Table~\ref{tab:frequency-ablation-five} reports the 5\% transition prior ablation.

\begin{table*}[t]
\centering
\footnotesize
\setlength{\tabcolsep}{4.1pt}
\caption{SLAKE official question group breakdown at 5\% keep ratio. Category definitions follow Table~\ref{tab:slake-main}. Avg. is the overall accuracy.}
\label{tab:slake-appendix-five}
\begin{tabular}{@{}clrrrrrr@{}}
\toprule
Model & Method & OR Acc.\(\uparrow\) & AB Acc.\(\uparrow\) & PO Acc.\(\uparrow\) & OT Acc.\(\uparrow\) & Avg. Acc.\(\uparrow\) & KL\(\downarrow\) \\
\midrule
\multirow{8}{*}{\rotatebox[origin=c]{90}{\scriptsize Lingshu-7B}}
& Full tokens & \stdcell{88.40}{0.95} & \stdcell{72.78}{1.74} & \stdcell{94.81}{2.53} & \stdcell{86.43}{1.51} & \stdcell{83.92}{0.75} & \stdcell{0.000}{0.000} \\
\cmidrule(lr){2-8}
& Random & \stdcell{54.23}{1.47} & \stdcell{26.45}{1.72} & \stdcell{51.95}{5.69} & \stdcell{62.02}{2.14} & \stdcell{48.25}{1.02} & \stdcell{0.758}{0.017} \\
& BTP & \stdcell{\underline{74.02}}{1.29} & \stdcell{\textbf{49.54}}{1.96} & \stdcell{\textbf{83.12}}{4.27} & \stdcell{\underline{72.48}}{1.97} & \stdcell{\underline{67.29}}{0.96} & \stdcell{\underline{0.341}}{0.012} \\
& FastV & \stdcell{63.38}{1.42} & \stdcell{25.54}{1.71} & \stdcell{58.44}{5.62} & \stdcell{65.70}{2.09} & \stdcell{53.38}{1.02} & \stdcell{0.587}{0.014} \\
& SparseVLM & \stdcell{63.64}{1.42} & \stdcell{26.45}{1.72} & \stdcell{64.94}{5.44} & \stdcell{67.25}{2.07} & \stdcell{54.30}{1.02} & \stdcell{0.555}{0.013} \\
& VisPruner & \stdcell{67.74}{1.38} & \stdcell{\underline{48.62}}{1.95} & \stdcell{75.32}{4.91} & \stdcell{69.96}{2.02} & \stdcell{63.24}{0.99} & \stdcell{0.441}{0.012} \\
& HRViT & \stdcell{64.95}{1.41} & \stdcell{28.29}{1.76} & \stdcell{66.23}{5.39} & \stdcell{68.02}{2.05} & \stdcell{55.64}{1.01} & \stdcell{0.531}{0.013} \\
& \method{} & \stdcell{\textbf{74.46}}{1.29} & \stdcell{47.71}{1.95} & \stdcell{\underline{81.82}}{4.40} & \stdcell{\textbf{81.98}}{1.69} & \stdcell{\textbf{69.01}}{0.95} & \stdcell{\textbf{0.336}}{0.013} \\
\midrule
\multirow{8}{*}{\rotatebox[origin=c]{90}{\scriptsize Qwen3-VL-8B}}
& Full tokens & \stdcell{85.61}{1.04} & \stdcell{65.75}{1.86} & \stdcell{94.81}{2.53} & \stdcell{83.72}{1.63} & \stdcell{80.08}{0.82} & \stdcell{0.000}{0.000} \\
\cmidrule(lr){2-8}
& Random & \stdcell{49.69}{1.48} & \stdcell{49.54}{1.96} & \stdcell{42.86}{5.64} & \stdcell{51.55}{2.20} & \stdcell{49.83}{1.02} & \stdcell{1.605}{0.044} \\
& BTP & \stdcell{\underline{68.96}}{1.37} & \stdcell{67.43}{1.83} & \stdcell{61.04}{5.56} & \stdcell{70.93}{2.00} & \stdcell{\underline{68.71}}{0.95} & \stdcell{\underline{0.703}}{0.029} \\
& FastV & \stdcell{62.16}{1.43} & \stdcell{64.53}{1.87} & \stdcell{\underline{66.23}}{5.39} & \stdcell{\underline{76.74}}{1.86} & \stdcell{66.08}{0.97} & \stdcell{0.759}{0.028} \\
& SparseVLM & \stdcell{68.00}{1.38} & \stdcell{64.22}{1.87} & \stdcell{\underline{66.23}}{5.39} & \stdcell{76.16}{1.88} & \stdcell{68.67}{0.95} & \stdcell{0.708}{0.028} \\
& VisPruner & \stdcell{66.78}{1.39} & \stdcell{\underline{68.04}}{1.82} & \stdcell{61.04}{5.56} & \stdcell{72.67}{1.96} & \stdcell{68.21}{0.95} & \stdcell{0.716}{0.030} \\
& HRViT & \stdcell{64.78}{1.41} & \stdcell{62.39}{1.89} & \stdcell{50.65}{5.70} & \stdcell{74.22}{1.93} & \stdcell{65.71}{0.97} & \stdcell{0.772}{0.029} \\
& \method{} & \stdcell{\textbf{76.55}}{1.25} & \stdcell{\textbf{68.50}}{1.82} & \stdcell{\textbf{71.43}}{5.15} & \stdcell{\textbf{77.91}}{1.83} & \stdcell{\textbf{74.48}}{0.89} & \stdcell{\textbf{0.494}}{0.025} \\
\bottomrule
\end{tabular}
\end{table*}

\begin{table*}[t]
\centering
\footnotesize
\setlength{\tabcolsep}{4.1pt}
\caption{OmniMedVQA semantic group breakdown at 5\% keep ratio. Category definitions follow Table~\ref{tab:omnimed-main}. Avg. is the overall accuracy.}
\label{tab:omnimed-appendix-five}
\begin{tabular}{@{}clrrrrrr@{}}
\toprule
Model & Method & OS Acc.\(\uparrow\) & RJ Acc.\(\uparrow\) & LC Acc.\(\uparrow\) & ES Acc.\(\uparrow\) & Avg. Acc.\(\uparrow\) & KL\(\downarrow\) \\
\midrule
\multirow{8}{*}{\rotatebox[origin=c]{90}{\scriptsize Lingshu-7B}}
& Full tokens & \stdcell{73.80}{1.15} & \stdcell{83.90}{1.20} & \stdcell{86.82}{1.19} & \stdcell{95.94}{1.78} & \stdcell{80.62}{0.69} & \stdcell{0.000}{0.000} \\
\cmidrule(lr){2-8}
& Random & \stdcell{20.10}{1.05} & \stdcell{58.58}{1.60} & \stdcell{26.99}{1.57} & \stdcell{65.04}{4.30} & \stdcell{34.33}{0.82} & \stdcell{1.149}{0.017} \\
& BTP & \stdcell{25.58}{1.14} & \stdcell{59.85}{1.60} & \stdcell{39.93}{1.73} & \stdcell{\textbf{81.30}}{3.52} & \stdcell{40.82}{0.85} & \stdcell{0.950}{0.016} \\
& FastV & \stdcell{16.53}{0.97} & \stdcell{53.28}{1.62} & \stdcell{24.63}{1.52} & \stdcell{61.79}{4.38} & \stdcell{30.58}{0.80} & \stdcell{1.143}{0.016} \\
& SparseVLM & \stdcell{16.80}{0.98} & \stdcell{54.77}{1.62} & \stdcell{27.61}{1.58} & \stdcell{62.60}{4.36} & \stdcell{31.87}{0.81} & \stdcell{1.126}{0.016} \\
& VisPruner & \stdcell{\underline{31.96}}{1.22} & \stdcell{\underline{65.78}}{1.54} & \stdcell{\underline{40.30}}{1.73} & \stdcell{\underline{69.11}}{4.17} & \stdcell{\underline{44.94}}{0.86} & \stdcell{\underline{0.928}}{0.017} \\
& HRViT & \stdcell{27.43}{1.17} & \stdcell{58.90}{1.60} & \stdcell{38.56}{1.72} & \stdcell{64.23}{4.32} & \stdcell{40.40}{0.85} & \stdcell{0.959}{0.015} \\
& \method{} & \stdcell{\textbf{60.29}}{1.28} & \stdcell{\textbf{76.59}}{1.38} & \stdcell{\textbf{62.31}}{1.71} & \stdcell{64.23}{4.32} & \stdcell{\textbf{65.55}}{0.82} & \stdcell{\textbf{0.427}}{0.012} \\
\midrule
\multirow{8}{*}{\rotatebox[origin=c]{90}{\scriptsize Qwen3-VL-8B}}
& Full tokens & \stdcell{56.24}{1.30} & \stdcell{84.43}{1.18} & \stdcell{70.52}{1.61} & \stdcell{69.11}{4.17} & \stdcell{68.16}{0.81} & \stdcell{0.000}{0.000} \\
\cmidrule(lr){2-8}
& Random & \stdcell{34.36}{1.24} & \stdcell{53.07}{1.62} & \stdcell{51.62}{1.76} & \stdcell{\underline{67.48}}{4.22} & \stdcell{45.06}{0.86} & \stdcell{1.690}{0.041} \\
& BTP & \stdcell{\textbf{37.11}}{1.27} & \stdcell{\underline{67.16}}{1.53} & \stdcell{\underline{54.35}}{1.76} & \stdcell{65.85}{4.28} & \stdcell{\underline{50.86}}{0.87} & \stdcell{\underline{1.232}}{0.037} \\
& FastV & \stdcell{35.19}{1.25} & \stdcell{59.85}{1.60} & \stdcell{50.75}{1.76} & \stdcell{\textbf{68.29}}{4.20} & \stdcell{47.16}{0.87} & \stdcell{1.519}{0.039} \\
& SparseVLM & \stdcell{33.47}{1.24} & \stdcell{63.35}{1.57} & \stdcell{\textbf{55.35}}{1.75} & \stdcell{66.67}{4.25} & \stdcell{48.45}{0.87} & \stdcell{1.513}{0.040} \\
& VisPruner & \stdcell{35.94}{1.26} & \stdcell{66.21}{1.54} & \stdcell{52.86}{1.76} & \stdcell{65.04}{4.30} & \stdcell{49.68}{0.87} & \stdcell{1.387}{0.039} \\
& HRViT & \stdcell{34.50}{1.24} & \stdcell{62.39}{1.58} & \stdcell{51.49}{1.76} & \stdcell{63.41}{4.34} & \stdcell{47.58}{0.87} & \stdcell{1.353}{0.039} \\
& \method{} & \stdcell{\underline{36.35}}{1.26} & \stdcell{\textbf{70.02}}{1.49} & \stdcell{\underline{54.35}}{1.76} & \stdcell{64.23}{4.32} & \stdcell{\textbf{51.28}}{0.87} & \stdcell{\textbf{1.230}}{0.037} \\
\bottomrule
\end{tabular}
\end{table*}

\begin{table*}[t]
\centering
\scriptsize
\setlength{\tabcolsep}{3.8pt}
\caption{Transition prior ablation with Lingshu-7B at 5\% keep ratio. The column order and category definitions match Table~\ref{tab:frequency-ablation}.}
\label{tab:frequency-ablation-five}
\begin{tabular}{@{}clrrrrrr@{}}
\toprule
Dataset & Variant & OR Acc.\(\uparrow\) & AB Acc.\(\uparrow\) & PO Acc.\(\uparrow\) & OT Acc.\(\uparrow\) & Avg. Acc.\(\uparrow\) & KL\(\downarrow\) \\
\midrule
\multirow{2}{*}{SLAKE} & w/o trans. & \stdcell{\underline{73.67}}{1.30} & \stdcell{\underline{45.72}}{1.95} & \stdcell{\textbf{81.82}}{4.40} & \stdcell{\underline{79.07}}{1.79} & \stdcell{\underline{67.46}}{0.96} & \stdcell{\underline{0.348}}{0.014} \\
& \method{} & \stdcell{\textbf{74.46}}{1.29} & \stdcell{\textbf{47.71}}{1.95} & \stdcell{\textbf{81.82}}{4.40} & \stdcell{\textbf{81.98}}{1.69} & \stdcell{\textbf{69.01}}{0.95} & \stdcell{\textbf{0.336}}{0.013} \\
\midrule
Dataset & Variant & OS Acc.\(\uparrow\) & RJ Acc.\(\uparrow\) & LC Acc.\(\uparrow\) & ES Acc.\(\uparrow\) & Avg. Acc.\(\uparrow\) & KL\(\downarrow\) \\
\midrule
\multirow{2}{*}{OmniMedVQA} & w/o trans. & \stdcell{\underline{59.14}}{1.25} & \stdcell{\underline{74.05}}{1.43} & \stdcell{\underline{56.50}}{1.86} & \stdcell{\underline{63.41}}{4.34} & \stdcell{\underline{62.96}}{0.84} & \stdcell{\underline{0.448}}{0.012} \\
& \method{} & \stdcell{\textbf{60.29}}{1.28} & \stdcell{\textbf{76.59}}{1.38} & \stdcell{\textbf{62.31}}{1.71} & \stdcell{\textbf{64.23}}{4.32} & \stdcell{\textbf{65.55}}{0.82} & \stdcell{\textbf{0.427}}{0.012} \\
\bottomrule
\end{tabular}
\end{table*}
